# Supplementary material for: Magnetization Reversal Across Multiple Serial Barriers in a Single Fe$_3$O$_4$ Nanoparticle
Source: arXiv:2201.09011 source file (2022-01-22)
Supplement: Supplementary file 1 [file suppl-info-SwitchingStatMS-Sagar-6.pdf]

# Supplementary information on "Magnetization reversal across multiple serial barriers in a single $Fe_3O_4$ nanoparticle" by S. Paul et. al.

There are five sections in this Suppl Info. The first section presents micro-magnetic Mumax simulations on magnetization reversal of a spherical nano-particle with uniaxial anisotropy. The 2nd section elaborates on experimental details, the 3rd section provides the mathematical details of serial barrier model, the 4th section presents a detailed comparison of serial barrier model with few other relevant distributions. The last section presents the analysis of permalloy nano-wires switching statistics using stretched exponential distribution and that arising from parallel barriers.

## 1 Micro-magnetic simulations on spherical nanoparticle

$Fe_3O_4$ undergoes a structural transition, namely the Verwey transition, in 80 - 120 K temperature range. The inverse spinel cubic structure at room temperature transforms into a orthorhombic one at low temperature. As a result, magneto-crystalline anisotropy [2] is believed to change from cubic at room temperatures to predominantly uniaxial at low temperatures. In the actual sample, there can be a few crystal grains; however, we assume an overall uniaxial anisotropy for a qualitative understanding using the micromagnetic simulations with Mumax [1].

The material parameters available in literature vary for different particle size and temperature [2]. Following are the material parameters used here for the micro-magnetic simulations: saturation magnetization, $M_s$ = 500 x $10^3$ A/m = 100 emu/gm with the density of $Fe_3O_4$ $\sim$ 5 gm/cm$^3$, exchange stiffness, $A_{ex} = 4 \times 10^{-12}$ J/m, effective uniaxial-anisotropy energy density, $K$ = 30000 J/m$^3$. The simulations were done with particle diameter 150 nm and with a finite-element cubic cell of side 3 nm. The field was applied along the x-axis which is the easy axis. The blue color in Fig. 1 shows the simulated $M - H$ loop compared to one of the experimental $M - H$ of $Fe_3O_4$ F#1. The simulation results are depicted in two different cross-section images of the spherical particle at 4 different values of the field. This reveals the magnetization reversal by a single vortex nucleation and annihilation.

## 2 Experimental Details

Magnetism of individual nano-structure was probed using externally shunted Nb $\mu$-SQUID working in a non-hysteretic regime. An optimized external shunt having both inductance and resistance was found to eliminate thermal hysteresis [3, 4] in the $I - V$ characteristics

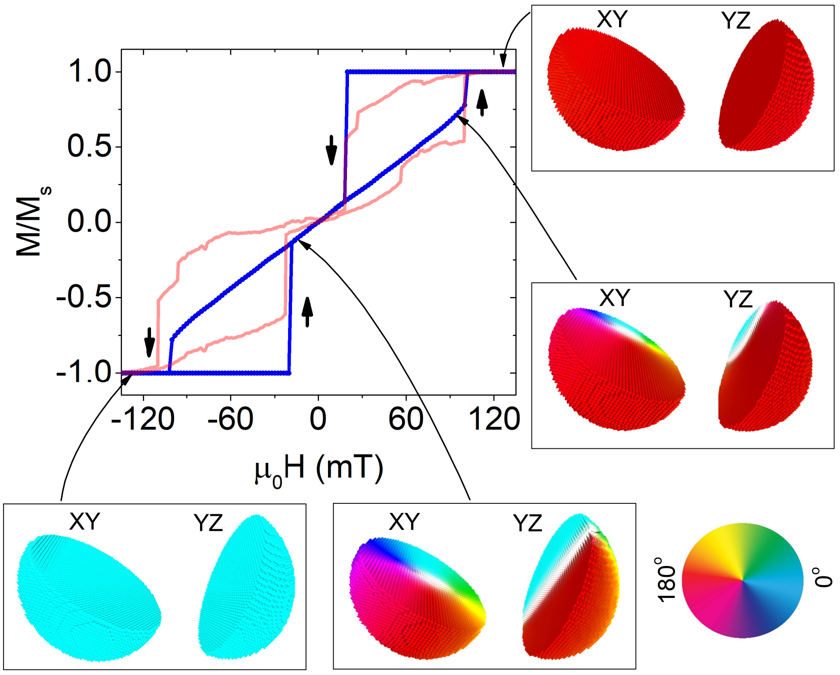


Figure 1: A comparison of Mumax simulation of $M-H$ loop (blue) for a spherical nanoparticle of diameter $\sim$ 150 nm as compared to the experimental $M-H$ loop (light red) of $Fe_3O_4$ F#1. The field is swept along x-axis, which is the easy axis. The simulation displays with two planar cross sections, xy (left hemisphere) yz (right hemisphere), of the particle with spin texture during vortex traversal. The color circle on bottom right shows the HSL (hue, saturation, lightness) color scheme for the spin component in xy-plane. The cyan color indicates spin along -x and red indicates spin along +x direction. The white color indicates spin along +z direction.

(IVC) of $\mu$-SQUIDs [5, 6]. The Nb $\mu$-SQUIDs were fabricated from a 20 nm thick Nb film using e-beam lithography as described in an earlier work [6] together with the details of the measurement setup including a 3D vector magnet and its successful use on permalloy nano-needles. Recently we have further refined the $\mu$-SQUID's performance by using a commercial low temperature SQUID-array amplifier leading to better sensitivity.

All magnetic measurements in this report were performed with external field aligned in the $\mu$-SQUID plane, using a 3D vector magnet. An optimally biased non-hysteretic $\mu$-SQUID eventually gives a nearly linear voltage readout of flux through the SQUID-loop and thus the magnetic response $M(H)$ of the particle is registered as a change in voltage $V(H)$. This voltage is scaled using two extreme voltages corresponding to two opposite saturation magnetization to obtain $M/M_s$ vs $H$ plots. The anisotropy in switching field $H_{sw}(\theta)$ is measured through in-plane angle $\theta$ dependent switching fields obtained from $M/M_s$ vs $H$ plots. Switching field histograms were obtained by repeated ramping of the field at fixed angle $\theta$ and at a specific rate and registering $H_{sw}$ at which the sharp jump occurs. Note that a $\mu$-SQUID working in this voltage read-out mode is capable of very fast response to magnetic signals and the measurement speed is limited mainly by the inductance of the magnet coils. Waiting time histograms were obtained by ramping the field up from below negative $H_w$ value to a fixed field $H_w$ just below $H_{sw}$ and noting the

time until switching, after arriving to $H_w$.

We present the magnetization reversal/ switching statistics of three $Fe_3O_4$ nanoparticles of size $\sim$ 150 nm [$F\#1-3$] and a permalloy nano-wire of size $\sim 2$ $\mu$m x (width) 80 nm x (thickness) 100 nm [$N\#1$] while similar behavior is observed in several other such objects. The magnetite ($Fe_3O_4$) nano-particles were synthesized using a simple polyol method. Weighted quantity of the precursor salt Iron nitrate nonahydrate, ($Fe(NO_3)_3{\cdot}9H_2O$ from Sigma Aldrich, was dissolved in a fixed volume of ethylene glycol (solvent) using magnetic stirrer. This solution was maintained at 160°C for about three hours for the reaction to occur till dark precipitates were obtained. The solution was decanted and the powder was washed several times using ethanol to remove the un-reacted salt. Subsequently the powder was allowed to dry in a vacuum furnace maintained at 120°C. Room temperature hysteresis measurements in a vibrating sample magnetometer (VSM) were performed on bulk powder form. These indicate soft ferromagnetic nature with coercivity $H_c = 235$ Oe and saturation magnetization $M_s = 67.8$ emu/gm. The former indicates a non-superparamagnetic character while the $M_s$ being smaller than the bulk value of 92 emu/gm shows a size smaller than bulk.

A substrate having several $\mu$-SQUIDs was dipped for a few seconds in Ethanol with dispersed $Fe_3O_4$ MNPs kept in a sonication bath. The substrate was then immediately placed on a permanent magnet for a fraction of second to avoid agglomeration of particles. Repeating this process a number of times yields few devices with single $Fe_3O_4$ at desired location. The success rate of this process is found to depend on the particle size, solvent type and surfactant. Permalloy nano-wires were fabricated by a e-beam lithography layer and precisely aligned with the existing $\mu$-SQUID [6].

# 3 Serial Barrier Model

For two barriers in series the overall probability of transition in time $t$ is the convolution of two PDFs: $p_i(t) = \tau_i^{-1}\exp(-t/\tau_i)$ $(i = 1, 2)$, given by $\int_0^t \int_0^{t-t_1} p_1(t_1)p_2(t_2)dt_2dt_1$. This is deduced by dividing the total time $t$ into $t_1$ & $t_2$ with no transition up to $t_1$ followed by first barrier crossing in interval $dt_1$, and then again no transition for time $t_2$ followed by the second barrier crossing in $dt_2$. For two unequal-transition-rate barriers, i.e. $\tau_1 \neq \tau_2$, this convolution works out as $P_{2u}(t) = (\tau_1 e^{-t/\tau_1} - \tau_2 e^{-t/\tau_2})/(\tau_1 - \tau_2)$. For the case of equal transition rates, $\tau_i^{-1} = \tau^{-1}$, for two barriers, the CDF of not switching works out as $P_{2e}(t) = (1 + \frac{t}{\tau})e^{-t/\tau}$ with mean switching time as $2\tau$.

For $N$ barriers with identical transition rates $\tau^{-1}$, the CDF for not switching is an $N$-fold convolution of $\exp(-t/\tau)$ which works out to be $P_{Ne}(t) = e^{-t/\tau}\sum_{k=0}^{N-1}\frac{(t/\tau)^k}{k!}$. The mean time to cross $N$ equal barriers works out as $\tau_{\text{eff}} = N\tau$. Not knowing $N$ *a priori*, but knowing $\tau_{\text{eff}}$, it is convenient to choose $\tau_{\text{eff}}$ as unit of time in above expression. This leads to $P_{Ne}(t) = e^{-Nt}\sum_{k=0}^{N-1}\frac{(Nt)^k}{k!}$. For $N$ *unequal* values of $\tau_i$, the CDF for not switching works out, from the convolution of $\exp(-t/\tau_i)$ functions, as

$$P_{Nu}(t) = \sum_i \frac{\tau_i^{N-1}}{f_i(\tau_1, \tau_2 ... \tau_N)} e^{-t/\tau_i}, \tag{1}$$

with $f_i(\tau_1, \tau_2 ... \tau_N) = \prod_{j\neq i}(\tau_i - \tau_j)$. In this case, the average time to overcome all the barriers is $\tau_{\text{eff}} = \sum_{i=1}\tau_i$.

# 4 Comparison of serial barriers with other relevant distributions

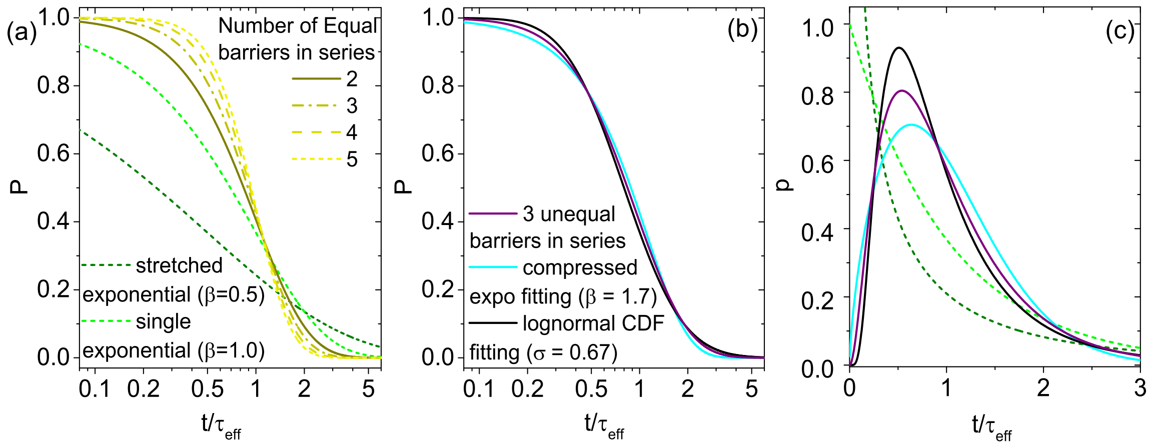


Figure 2: (a) CDF of N (=2-5) equal barrier model plotted with scaled time for different values of N together with an exponential and stretched exponential ($\beta = 0.5$) for comparison. (b) shows the CDF of three unequal serial barrier model and compared to compressed exponential ($\beta = 1.7$) and CDF of log-normal with $\sigma = 0.67$. (c) shows the corresponding PDFs.

Fig. 2(a) shows the CDF for $N$ equal barrier model, i.e. $P_{Ne}(t) = e^{-Nt/\tau_{eff}} \sum_{k=0}^{N-1} \frac{(Nt/\tau_{eff})^k}{k!}$ plotted with a scaled time $t/\tau_{eff}$ for different values of $N$. Here $\tau_{eff} = N\tau$ is the effective mean time of crossing $N$ equal barriers. For larger values of $N$ the CDF declines more sharply and hence the corresponding PDF is narrower. The width of the PDF is proportional to $\tau_{eff}/\sqrt{N}$.

A commonly used relaxation function is a modified exponential function given by $P_W(t) = \exp[-(t/\tau)^\beta]$ with the PDF $p_W(t) = (\beta t^{\beta-1}/\tau^\beta)\exp\left[-(t/\tau)^\beta\right]$. This is known as Weibull distribution and it encompasses: a) the common exponential ($\beta = 1$), b) the stretched exponential ($\beta < 1$) and c) the compressed exponential ($\beta > 1$). The mean switching time here is given by $\tau_{eff} = \tau\Gamma(1 + 1/\beta)$. The stretched exponential ($\beta < 1$) derives its justification from a distribution of parallel barriers.

The log-normal distribution is another distribution which matches fairly well with both the compressed exponential and the serial barrier scenario. The CDF for not-switching for the log-normal is given by,

$$P_L(t) = \frac{1}{2} - \frac{1}{2}\text{erf}\left[\frac{\ln(t/\tau_0)}{\sqrt{2}\sigma}\right]. \tag{2}$$

Here $\ln\tau_0$ and $\sigma$ are the mean and the standard deviation of $\ln t$, respectively. The mean switching time for this distribution is $\tau_{\text{eff}} = \tau_0\exp(\sigma^2/2)$. Log-normal distribution has been used to describe multiplicative processes [7, 8, 9] and it can be derived from central limit theorem for multiplicative variables [9].

Figure 2(b) shows a comparison between the compressed exponential, log-normal and the serial barrier model. The experimental CDF for F#1, 3 were also fitted to the log-

normal CDF and compressed exponential other than unequal serial barriers. The evolution of the fitting parameters and reduced-$\chi^2$ for the three cases is given in Table 1.

Table 1: Fitting parameters for CDF for not switching for different $H_w$ for $Fe_3O_4$ devices. Here, $X = \chi_r^2 \times 10^4$, $\tau_{\rm eff}$ is the effective mean switching time. Note that $\tau_{eff}$ from different fits are similar for a given $H_w$ and $\tau_{eff}$ decreases rapidly with increasing field. Also $\beta$ decreases and $\sigma$ increases with increasing $\mu_0 H_w$.

| Device no. | $\mu_0 H_w$ (mT) | Compressed expo. | | | Lognormal CDF | | | 3 Unequal Barriers | |
|---|---|---|---|---|---|---|---|---|---|
| | | $\beta$ | $\tau_{eff}(s)$ | X | $\sigma$ | $\tau_{eff}(s)$ | X | $\tau_{eff}(s)$ | X |
| F#1 | 100.00 | 1.16 | 12.19 | 7.9 | 0.87 | 13.05 | 2.8 | 12.43 | 4.5 |
| | 100.20 | 1.36 | 3.06 | 1.3 | 0.76 | 3.25 | 2.6 | 3.13 | 0.7 |
| | 100.40 | 1.24 | 1.03 | 1.2 | 0.83 | 1.11 | 4.0 | 1.06 | 1.2 |
| | 100.45 | 1.00 | 0.22 | 2.3 | 1.06 | 0.25 | 2.8 | 0.21 | 4.7 |
| F#3 | 129.20 | 1.71 | 25.37 | 12.1 | 0.67 | 24.64 | 0.7 | 27.56 | 2.1 |
| | 129.50 | 1.66 | 8.25 | 11.2 | 0.81 | 9.86 | 0.5 | 8.88 | 0.8 |
| | 129.65 | 1.55 | 4.14 | 17.6 | 0.89 | 4.65 | 0.9 | 4.62 | 2.6 |
| | 129.80 | 1.00 | 1.24 | 1.3 | 1.04 | 1.41 | 1.7 | 1.25 | 1.3 |

# 5 Parallel barriers in permalloy nanowire

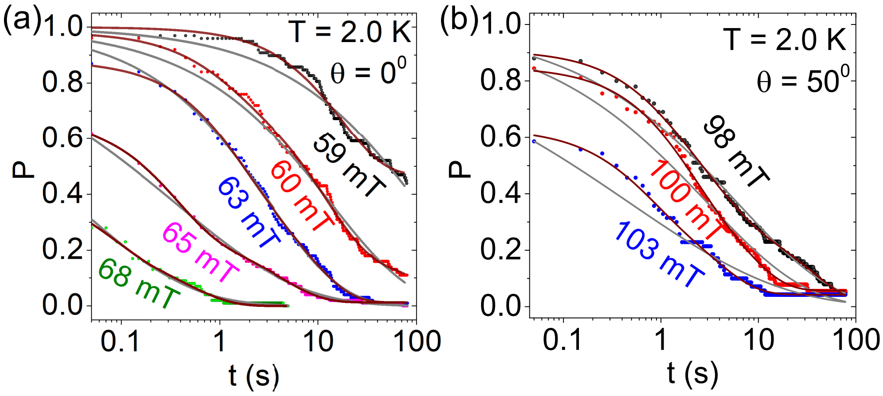


Figure 3: The probability of not switching (P) vs time (t) obtained at 2.0 K temperature for different fields (close to thermodynamic switching field) applied at angles (a) $\theta = 0$ and (b) 50° with respect to the easy axis for permalloy needle $N\#1$. The dark red lines show the fits to few parallel barrier model and the grey lines are the fits to stretched exponential.

Figure 3 shows the experimentally measured CDF of not-switching, i.e. $P(t)$, for a permalloy nanowire $N\#1$ obtained by integrating the waiting time histograms (with $\sim$ 100 counts). These are shown at 2.0 K temperature and for different waiting fields $H_w \lessapprox H_{\rm sw}$ applied at angle $\theta$ with respect to the needle axis which is the magnetic easy

axis. The anisotropy here is dictated by the shape. The switching field anisotropy in this case was found to be consistent with the curling mode as well as micro-magnetic simulations [6]. Best fits to both the stretched exponential, see Eq. 2, and three parallel barrier model, see Eq. 1, are also shown. The equation numbers here refer to the main paper. Clearly, the parallel barrier model fits are much better. It should be noted that we can fit the parallel-barrier model only for the paths for which the $\tau_i$s are within or close to the experimentally measured time range which actually extends from 50 ms to 100 s, see Fig. 3. The experimental switching data are acquired over a time range $t_{\min} \leq t \leq t_{\max}$ with a general measured histogram of waiting times exhibiting peaks at $t_{\min}$ and $t_{\max}$. This will be the case unless all $\tau_i$s are well within $t_{\min}$ and $t_{\max}$. These peaks represent cumulative switching events due to waiting times below $t_{\min}$ and above $t_{\max}$.

Table 2 shows the $\mu_0 H_w$ evolution of $\tau_i$'s and $w_i$'s of the three parallel barrier model for N#1 together with the stretched exponential fitting parameters. Note that in some cases, one of the mean times goes beyond our measurement time window. In such cases, one gets either a considerably large count of switching events at zero time, corresponding to already switched in less than least measurable time, or no switching up to the maximum waiting time. But one should not ignore this data since they contribute to the weight $w$'s as we see in this table (also see in Fig. 3 that at extreme waiting times some of the curves do not saturate to 0 or 1 yet). The three parallel paths fit the experimental data considerably better than the stretched exponential.

Table 2: Fitting parameters for CDF of not switching for different $H_w$ for permalloy nanowire N#1.

| $T$, $\theta$ | $\mu_0 H_w$ (mT) | Stretched expo. | | 3 Parallel Barriers | | |
|---|---|---|---|---|---|---|
| | | $\beta$ | $\tau(s)$ | $\tau_1(s)$, $w_1$ | $\tau_2(s)$, $w_2$ | $\tau_3(s)$, $w_3$ |
| 2.0 K, 0° | 59.0 | 0.54 | 102.63 | | 17.90, 0.53 | >200, 0.47 |
| | 60.0 | 0.53 | 13.50 | 1.13, 0.20 | 11.69, 0.60 | 149.4, 0.19 |
| | 63.0 | 0.59 | 3.23 | <0.03, 0.12 | 1.28, 0.38 | 7.89, 0.49 |
| | 65.0 | 0.34 | 0.36 | <0.03, 0.33 | 0.34, 0.41 | 4.08, 0.25 |
| | 68.0 | 0.37 | 0.03 | <0.03, 0.57 | 0.07, 0.23 | 0.49, 0.20 |
| 2.0 K, 50° | 98.0 | 0.44 | 6.10 | 0.91, 0.20 | 3.42, 0.42 | 36.32, 0.35 |
| | 100.0 | 0.43 | 3.01 | <0.03, 0.15 | 1.51, 0.35 | 6.76, 0.44 |
| | 103.0 | 0.28 | 0.48 | <0.03, 0.37 | 0.60, 0.25 | 3.60, 0.34 |
| 4.0 K, 0° | 58.0 | 0.24 | 0.94 | <0.03, 0.28 | 1.77, 0.58 | 92.39, 0.13 |
| | 65.0 | 0.21 | 0.01 | <0.03, 0.72 | 0.43, 0.22 | 4.41, 0.05 |

Switching field histograms in permalloy N#1 also show multiple peaks or multiple merged histograms as shown in Fig. 4. This arises from different switching fields for different parallel pathways indicating parallel paths. Similar feature was also observed in other systems like Ni nanowire [10]. In few occasions we could also identify two parallel paths directly in $M - H$ loops of permalloy nanowire.

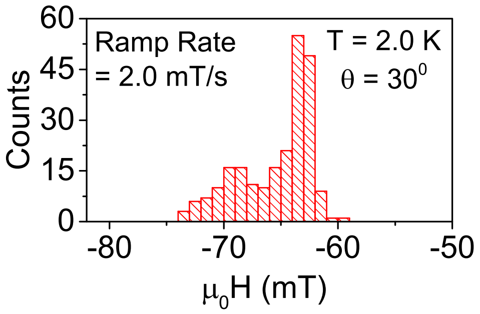


Figure 4: (a) Switching field histogram of permalloy nanowire for magnetic field applied at 30° angle with easy axis and displaying multiple merged peaks.

# References

[1] "The design and verification of MuMax3", A. Vansteenkiste, J. Leliaert, M. Dvornik, M. Helsen, F. Garcia-Sanchez, and B. V. Waeyenberge, AIP Advances **4**, 107133 (2014)

[2] "Spin disorder and magnetic anisotropy in Nanoparticles", E. Lima, A. L. Brandl, A. D. Arelaro, and G. F. Goya, J. Appl. Phys. **99**, 083908 (2006).

[3] "Reversibility of Superconducting Nb Weak Links Driven by the Proximity Effect in a Quantum Interference Device", N. Kumar, T. Fournier, H. Courtois, C. B. Winkelmann and Anjan K. Gupta, Phys. Rev. Lett. **114**, 157003 (2015).

[4] "Josephson coupling in the dissipative state of a thermally hysteretic micro-SQUID", S. Biswas, C. B. Winkelmann, H. Courtois, and Anjan K. Gupta, Phys. Rev. B **98**, 174514 (2018).

[5] "Elimination of thermal hysteresis with large V-$\phi$ transduction in $\mu$-SQUIDs by inductive shunt", S. Biswas, C. B. Winkelmann, H. Courtois, and A. K. Gupta, Phys. Rev. B **101**, 024501 (2020).

[6] "Probing magnetism of individual nano-structures using Nb $\mu$-SQUIDs in hysteresis free mode", S. Paul, G. Kotagiri, R. Ganguly, H. Parashari, H. Courtois, C. B. Winkelmann, A. K. Gupta, J. Magn. Magn. Mater. **503** (2020) 166625.

[7] "On the Statistics of Individual Variations of Productivity in Research Laboratories", W. Shockley, Proc. IRE **45**, 279 (1957).

[8] "On 1/f noise and other distributions with long tail", E. W. Montroll and M. F. Shlesinger, Proc. Nat. Acad. Sci. **79**, 3380 (1982).

[9] "On relaxations and aging of various glasses", A. Amira, Y. Orega, and Y. Imry, Proc. Nat. Acad. Sci. **109**, 1850 (2012).

[10] "Nucleation of Magnetization Reversal in Individual Nanosized Nickel Wires", W. Wernsdorfer, B. Doudin, D. Mailly, K. Hasselbach, A. Benoit, J. Meier, J. -Ph. Ansermet, and B. Barbara, Phys. Rev. Lett. **77**, 1873 (1996).
